# Supplementary material for: Towards self dual Loop Quantum Gravity
Source: arXiv:1511.07332 source file (2015-11-23)
Supplement: Supplementary file 1 [file Appendices.tex]

\documentclass[../PhD_thesis.tex]{subfiles}

\def\be{\begin{equation}}
\def\ee{\end{equation}}   
\def\ba{\begin{eqnarray}}
\def\ea{\end{eqnarray}}
\def\bas{\begin{subequations}\begin{eqnarray}}
\def\eas{\end{eqnarray}\end{subequations}}

\def\eps{\varepsilon}

\def\de{\mathrm{d}}

\def\f{\frac}

\def\su{\mathfrak{su}}
\def\so{\mathfrak{so}}

\def\time{\,{\scriptstyle{\times}}\,}

\begin{document}

\section{Black Holes}

\subsection{First law of thermodynamics for weakly isolated horizons}

Let us derive this first law. We assume that the boundary condition at infinity are asymptotic flatness and that our (weakly) isolated horizon have a vanishing angular momentum. The case of rotating IH have been studied in []. We denote $\Gamma$ the phase space of General Relativity supplemented with the weaky isolated horizon boundaries conditions. A point of this phase space is coordinated by the two fields $(\Sigma, K)$ where $\Sigma_{i} = \epsilon_{ijk} e^{j}\wedge e^{k}$ is the electric field and $K^{i} = \omega^{0i}$ is the extrinsic curvature. 

In order to derive the first law of thermodynamics, we have to pick up an evolution vector field denoted $t^{a}$  on the manifold $\mathcal{M}$.
This vector field on the manifold defines another vector field $\delta_{t}$ which lives on the phase space $\Gamma$. For the connection $A$ and the electric field $\Sigma$, we have: $\delta_{t} =( \mathcal{L}_{t} K, \mathcal{L}_{t} \Sigma)$.
This vector field has to be interpreted as the infinitesimal generators of tie evolution on the covariant phase space. Now, we require that the vector be hamiltonian, i.e. that it generates a phase space symmetry.
This is the case if the Lie derivative of the symplectic two form is vanishing everywhere on the phase space, i.e. $\mathcal{L}_{t} \Omega = 0$.
The necessary and sufficient condition for this to happen is that there exists a function $H_{t}$ such that:
\begin{align}
\delta H_{t} = \Omega(\delta, \delta_{t}) \;\;\;\;\; \forall \delta \in \Gamma
\end{align}
We have now to specify the required boundary conditions on $t^{a}$ in order to satisfy the precedent equation.
Assuming asymptotic flatness at infinity, we require that $t^{a}$ approach a time translational Killing field of the flat Minkowski metric in this region.
At the horizon $\triangle$, there is no Killing field and the metric is not specified. However, a weakly isolated horizon is defined as a null $2+1$ manifold equipped with an equivalence class of null tangent vectors $[\chi]$.
Is is natural to require at the horizon that $t^{a}$ belongs to this equivalence class, i.e. $t^{a}|_{\triangle} \in [\chi]$.
Being interested in the evolution of the fields $(\Sigma, K)$ on the horizon, we set $t = \chi$.
To obtain the expression of the function $H_{t} = H_{\chi}$, we have compute the one form:
\begin{align*}
X_{\chi} (\delta) = \Omega(\delta, \delta_{\chi})
\end{align*}
If $X_{\chi}$ is a closed one form, then $dX_{\chi} = 0$ and we have: $X_{\chi} = d H_{\chi}$.
The explicit expression of $\delta_{\chi} K$  and $\delta_{\chi} \Sigma$ are:
\begin{align*}
\delta_{\chi} K & = \mathcal{L}_{\chi} K = [i_{\chi}, d] K = \chi. (dK) + d(\chi.K) \\
\delta_{\chi} \Sigma & = \mathcal{L}_{\chi} \Sigma = [i_{\chi}, d] \Sigma = \chi. (d\Sigma) + d(\chi.\Sigma) \\
\end{align*}
Using this formulas, we have for the one form $X_{\chi} (\delta)$:
\begin{align*}
X_{\chi} (\delta) = \Omega(\delta, \delta_{\chi}) = \int_{M} \delta_{\chi} \Sigma \wedge \delta K - \delta \Sigma \wedge \delta_{\chi} K
\end{align*}

\section{The Lie algebras $\boldsymbol{\su(2)}$, $\boldsymbol{\sl(2,\mathbb{C})}$, and $\boldsymbol{\su(1,1)}$}

\noindent Let us first introduce the two-dimensional traceless Hermitian Pauli matrices
\be
\sigma_1=
\begin{pmatrix}
0	&	1	\\
1	&     0 
\end{pmatrix},\qquad
\sigma_2=
\begin{pmatrix}
0	&	-\mathrm{i}	\\
\mathrm{i}	&     0 
\end{pmatrix},\qquad
\sigma_3=
\begin{pmatrix}
1	&	0	\\
0	&     -1 
\end{pmatrix},
\ee
which form a basis of the Lie algebra $\su(2)$. One choice of basis for $\sl(2,\mathbb{C})$ is given by the rotation generators $J_i=-\mathrm{i}\sigma_i/2$ and the boost generators $P_i=-\sigma_i/2=-\mathrm{i}J_i$, with $i=\{1,2,3\}$. They satisfy the following commutation relations:
\be\label{so(eta) basis}
[J_i,J_j]=\eps_{ij}^{~~k}J_k,\qquad[P_i,P_j]=-\eps_{ij}^{~~k}J_k,\qquad[P_i,J_j]=\eps_{ij}^{~~k}P_k.
\ee
One can see that the rotational algebra $\su(2)$ generated by the elements $J_i$ forms a subalgebra of the algebra $\sl(2,\mathbb{C})$. On the other hand, the subalgebra $\su(1,1)$ is generated by the elements $(J_3,P_1,P_2)$, and one can see from (\ref{so(eta) basis}) that their commutation relations are given by 
\be
[P_1,P_2]=-J_3,\qquad
[P_2,J_3]=P_1,\qquad
[J_3,P_1]=P_2.
\ee
In the literature, the Lie algebra $\su(1,1)$ is often defined as being generated by the three elements
\be
F_0=
\f{1}{2}\begin{pmatrix}
-1	&	0	\\
0	&     1 
\end{pmatrix},\qquad
F_1=
\f{\mathrm{i}}{2}\begin{pmatrix}
0	&	1	\\
1	&     0 
\end{pmatrix},\qquad
F_2=
\f{1}{2}\begin{pmatrix}
0	&	1	\\
-1	&     0 
\end{pmatrix},
\ee
which satisfy the commutation relations
\be
[F_1,F_2]=\mathrm{i}F_0,\qquad
[F_0,F_2]=\mathrm{i}F_1,\qquad
[F_0,F_1]=-\mathrm{i}F_2.
\ee
These generators are related to the previous ones through the map $(J_3,P_1,P_2)\longmapsto\mathrm{i}(F_0,F_1,F_2)$.

Now, starting from the basis (\ref{so(eta) basis}), it is convenient to define a new basis $T_i^\pm$ as
\be
T_i^\pm\equiv\f{1}{2}(J_i\pm\mathrm{i}P_i),
\ee
whose generators realize two commuting copies of $\su(2)$, i.e. satisfy
\be
[T_i^\pm,T_j^\pm]=\eps_{ij}^{~~k}T_k^\pm,\qquad[T_i^+,T_j^-]=0.
\ee
Anti-symmetric bivectors $B^{IJ}$ form the adjoint representation of $\so(3,1)$. The Hodge duality operator acts on them as
\be
\star B^{IJ}=\f{1}{2}\eps^{IJ}_{~~KL}B^{KL},
\ee
which implies that $\star^2=-\text{id}$. We can therefore split the space of bivectors into the direct sum of two eigenspaces associated to the eigenvalues $\pm\mathrm{i}$, and write
\be
B^{IJ}=B^+_iT^{+IJ}_i+B^-_iT^{-IJ}_i.
\ee
The action of the Hodge dual on the (anti) self-dual components is given by
\be
\star B^\pm=\pm\mathrm{i}B^\pm,
\ee
and the vector representation of $\so(\eta)$ that we use is
\be
T^{\pm IJ}_i=\f{1}{2}\Big(\eps^{0iIJ}\pm\mathrm{i}\big(\eta^{0I}\eta^{iJ}-\eta^{iI}\eta^{0J}\big)\Big),
\ee
where $\eta^{IJ}=\text{diag}(-1,1,1,1)$.

\section{Commutator of two Ashtekar-Barbero connections}
\label{appendix:poisson}

\noindent The existence of the connection $\mathbf{A}$ (\ref{complex conn}) is a crucial point in the construction of section \ref{sec:quantum theory}. We have argued that this connection, shifted with a suitable term proportional to the Gauss constraint to give (\ref{asd}),  is canonically conjugated to the electric field $E$ (up to a global multiplicative factor). This argument relies on the fact that the shifted connection (\ref{asd}) corresponds to the self-dual or anti self-dual part of the initial $\sl(2,\mathbb{C})$ connection, which is itself conjugated to $E$. The non-trivial statement is that all the connections of the family (\ref{A and E}) (for any value of $\gamma$, either complex or real) are commutative. This can be proved by following the same reasoning as in the four-dimensional case and using properties of the components $\omega^i_a$ once the second class constraints are solved.

Due to the expression (\ref{asd}) where $\omega^i_a$ depends only on the variable $E^a_i$, showing that $\{A^i_a(x),A^j_b(y)\}=0$ reduces to the problem of showing that
\be
\{\omega_a^{(0)i}(x),\omega_b^j(y)\}+\{\omega_a^i(x),\omega_b^{(0)j}(y)\}=0,
\ee
for $a,b\in\{1,2\}$, $i,j\in\{1,2,3\}$ and $x,y\in\Sigma$, which in turn can be written as the condition
\be\label{crochetAG}
\{A_a^i(x),\omega_b^j(y)\}+\{\omega_a^i(x),A_b^j(y)\}=0,
\ee
since $\omega^i_a$ commutes with itself. To avoid a direct calculation of this relation, we proceed as in four dimensions, and look for a generating functional $W[E]$ depending on the variable $E$ only and such that $\omega_a^i(x)=\delta W[E]/\delta E^a_i(x)$. If this object exists, then the condition (\ref{crochetAG}) reduces to an integrability condition and follows immediately due to the fact that
\ba
\{A_a^i(x),\omega_b^j(y)\}+\{\omega_a^i(x),A_b^j(y)\}&=&\gamma\delta^2(x-y) 
\left(\frac{\delta\omega_a^i(x)}{\delta E^c_k(x)}\frac{\delta A_b^j(y)}{\delta A_c^k(y)}
-\frac{\delta A_a^i(x)}{\delta A_c^k(x)}\frac{\delta\omega_b^j(y)}{\delta E^c_k(y)}\right)\nonumber\\
&=&\gamma\delta^2(x-y) \left( \frac{\delta^2 W}{\delta E^a_i(x) \delta E^b_j(x)} - \frac{\delta^2 W}{\delta E^b_j(x) \delta E^a_i(x)} \right)\nonumber\\
&=&0.
\ea
For the generating functional we take
\be
W[E]=\int\de^2x\,E^a(x)\cdot\omega_a(x),
\ee
exactly as in four dimensions with the difference that now $\omega^i_a$ is given by (\ref{sol omega}):
\be
\omega_a=u\time\partial_au+\frac{1}{|E|}\eps_{ab}(E^b\cdot\partial_c E^c)x.
\ee
For the functional $W$ to be such that $\omega_a^i(x)=\delta W[E]/\delta E^a_i(x)$, it should satisfy
\be
\int\de^2x\ E^a(x)\cdot\delta\omega_a(x)=0
\ee
for any variation $\delta\omega$ of $\omega$, which implies that
\be
\delta W=\int\de^2x\,(\delta E^a\cdot\omega_a+E^a\cdot\delta\omega_a)=
\int\de^2x\,\delta E^a\cdot\omega_a.
\ee
For this to be true, we assume that the spatial slice $\Sigma$ has no boundaries. The proof uses the fact that $\omega^i_a$ satisfies
\be\label{properties of omega}
\partial_aE^a-\omega_a\time E^a=0,\qquad\partial_au-\omega_a\time u=0.
\ee
Therefore, we have
\ba
\int\de^2x\,E^a\cdot\delta\omega_a&=&\int\de^2x\,E^a\cdot\left[\delta(u\time\partial_au)+
\delta\left(\frac{1}{|E|}\eps_{ab}E^b\cdot\partial_cE^cx\right)\right]\nonumber\\
&=&\int\de^2x\,E^a\cdot\left(\delta u\time\partial_au+u\time\partial_a\delta u+\frac{1}{|E|}\eps_{ab}E^b\cdot\partial_cE^c\delta x\right),\label{blabla}
\ea
where we used the fact that $x\cdot E^a=0$. The first two terms between parenthesis above can now be written as follows:
\ba
\int\de^2x\,\delta u\cdot\big(\partial_au\time E^a-\partial_aE^a\time u-E^a\time\partial_au\big)
&=&\int\de^2x\,\delta u\cdot\big(2(\omega_a\time E^a)u-(\omega_a\cdot u)E^a\big)\nonumber\\
&=&-\int\de^2x\,\delta u\cdot E^a(\omega_a\cdot u)\nonumber\\
&=&-\int\de^2x\,\frac{1}{|E|}E^a\cdot\delta x\eps_{ab}E^b\cdot\partial_cE^c,
\ea
from which (\ref{blabla}) vanishes as announced. Notice that from the first to the second line we used the properties (\ref{properties of omega}) to replace the derivatives $\partial_a E^a$ and $\partial_a u$ by expressions involving $\omega$.

\end{document}
